# Supplementary material for: HEAD: HEtero-Assists Distillation for Heterogeneous Object Detectors
Source: arXiv:2207.05345 source file (2022-07-12)
Supplement: Supplementary file 1 [file comparison_to_kd_methods_with_assistants.tex]

TAKD~\cite{takd} employs intermediate-sized networks (teacher assistants) to improve the effectiveness of knowledge distillation between the teacher and student networks when the capacity (accuracy) gap is large. 
In HEAD, we adopt an assistant as the bridge between the student and teacher detectors. The assistant is homogeneous with the teacher head while sharing the backbone with the student, which is similar to the teacher assistant networks used in TAKD. 
Different from TAKD, which aims at bridging the capacity (accuracy) gap between homogeneous networks using the intermediate-sized networks, our approach adopts the assistant to solve the heterogeneity between detector pairs. 
Moreover, TAKD trains the intermediate-sized networks sequentially, which causes significant training time costs. In contrast, our assistant predictors are trained in an online distilling strategy, which is more efficient.

From another perspective, RCO~\cite{rco} supervises the student network with different checkpoints of the teacher model, which is similar to the teacher assistant networks used in TAKD. The checkpoints are saved per epoch during the training process of the teacher model. To find the optimal checkpoint for the student network to learn, RCO proposes a greedy search strategy. Similarly, our HEAD framework uses assistants to supervise the student predictor. Since our assistant predictors are trained in an online distillation strategy, the performance gap between the assistant and the student is always kept small. Therefore, the searching strategy in RCO becomes redundant for our framework.
