# Supplementary material for: HEAD: HEtero-Assists Distillation for Heterogeneous Object Detectors
Source: arXiv:2207.05345 source file (2022-07-12)
Supplement: Supplementary file 2 [file generating_proposals_with_one_stage_students.tex]

When the teacher is a two-stage detector and the student is a one-stage detector, our HEAD framework uses the student head to generate proposals. As an example, let the student be RetinaNet. Denote $\bm{R}^S \in \mathbb{R}^{4 \times A \times H \times W}$ and $\bm{C}^S \in \mathbb{R}^{K \times A \times H \times W}$ as the regression and classification outputs respectively, where $A$ is the number of anchors per location, $K$ is the number of classes, $H$ and $W$ represent the height and width respectively. $\bm{C}^S$ represents the classification \textit{logits} of each anchor, so its values are not bounded in the range $[0, 1]$. We first convert $\bm{C}^S$ to a class-agnostic objectness logit $\bm{O}^S \in \mathbb{R}^{A \times H \times W}$, where
\begin{equation}
  \bm{O}^S_{a, h, w} = \max_{k = 1, 2, \cdots, K} \bm{C}^S_{k, a, h, w},
\end{equation}
where $k$, $a$, $h$, and $w$ are the indices of the corresponding dimensions of $\bm{C}$.

Then we follow the original RPN protocol to generate RoIs. Specifically, we choose $2,000$ anchors with the highest objectness logits from the $A \times H \times W$ anchors. According to $\bm{R}^S$, we then map the $2,000$ anchors to $2,000$ proposals. 
Note that the $2,000$ proposals is generated for each FPN~\cite{fpn} level. We apply NMS on the union of these proposals. The IoU threshold of NMS is set to $0.7$. After NMS, the number of proposals is significantly reduced. If the number of proposals is still larger than $1,000$, we only keep the $1,000$ proposals with the highest objectness logits.
