# Supplementary material for: HEAD: HEtero-Assists Distillation for Heterogeneous Object Detectors
Source: arXiv:2207.05345 source file (2022-07-12)
Supplement: Supplementary file 3 [file visualization_of_backbone_features.tex]

\begin{figure*}
  \centering
  \includegraphics[width=\linewidth]{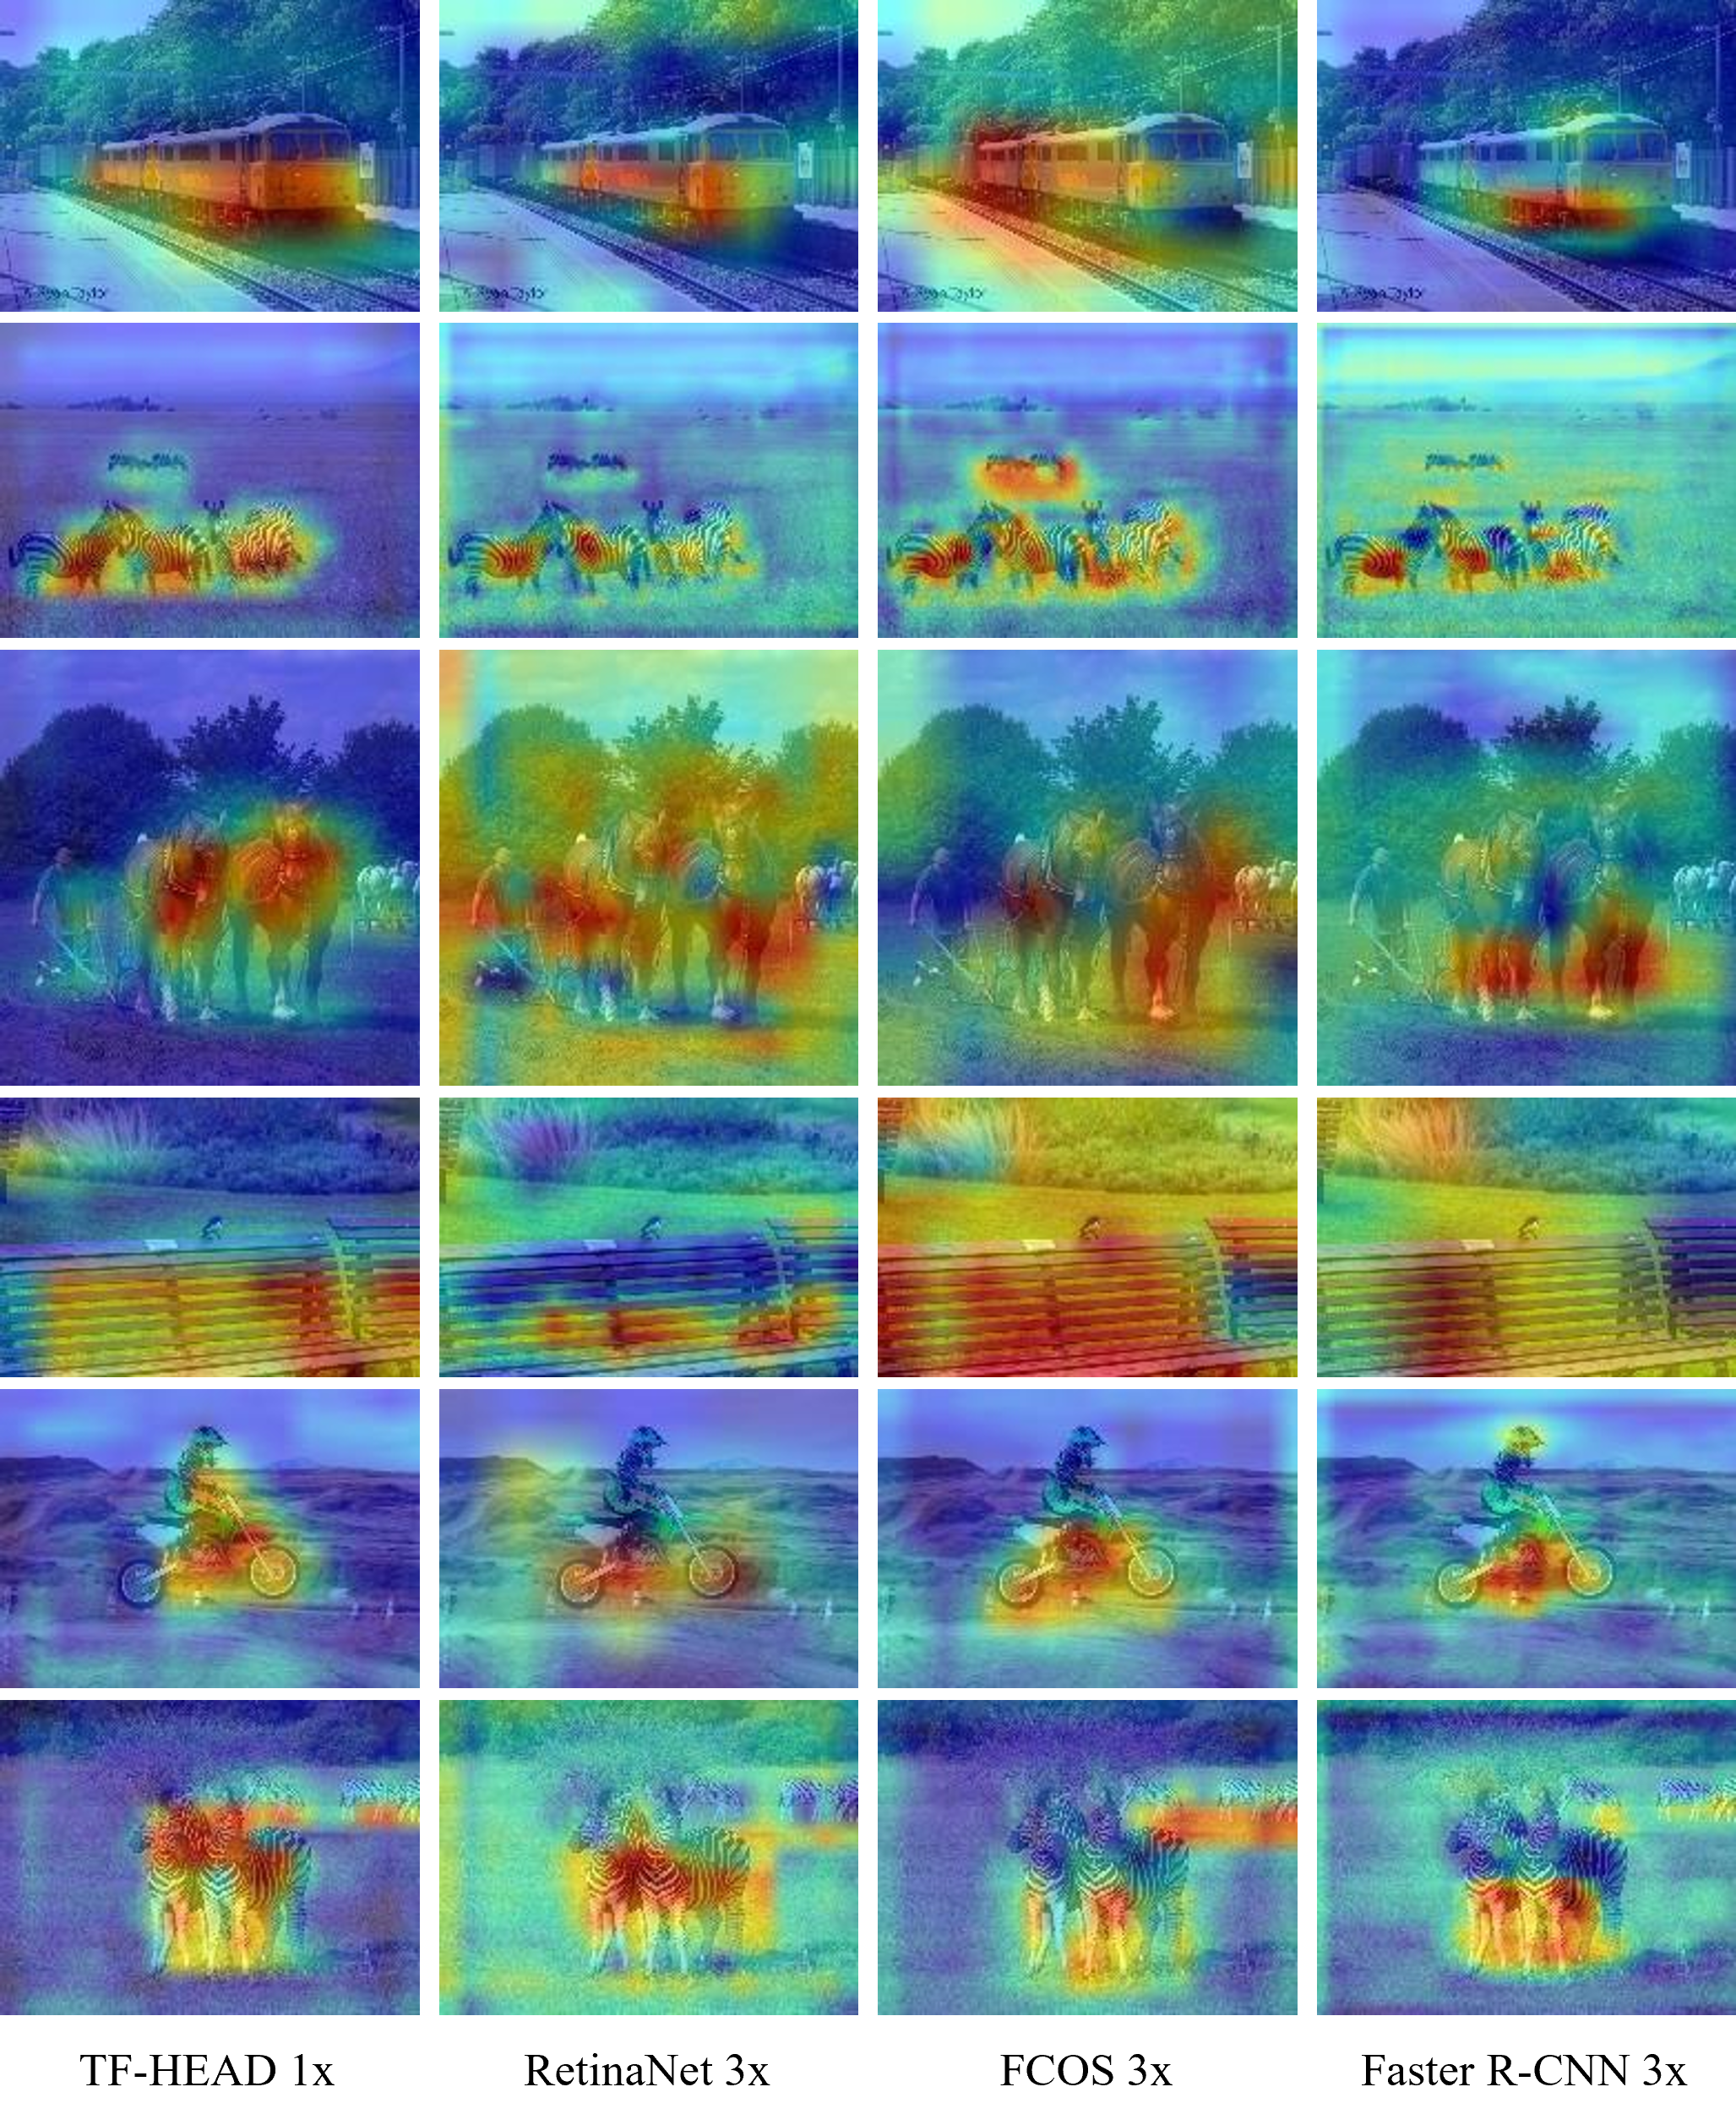}
  \caption{More visualizations of backbone features from TF-HEAD, RetinaNet~\cite{retinanet}, FCOS~\cite{fcos}, and Faster R-CNN~\cite{faster_rcnn}. }
  \label{fig:supp-vis}
\end{figure*}

In Fig.~\ref{fig:supp-vis}, we show more backbone features from TF-HEAD, RetinaNet~\cite{retinanet}, FCOS~\cite{fcos}, and Faster R-CNN~\cite{faster_rcnn}. The visualized feature maps are outputs of FPN~\cite{fpn}, where feature levels are chosen according to the size of target. Let $\bm{P} \in \mathbb{R}^{C \times H \times W}$ denote the feature map to be visualized, where $C$ is the channel number, $H$ and $W$ represent the height and width respectively. $\bm{P}$ is first reduced to a 2-dimensional heatmap and then converted to gray-scale by the following steps
\begin{eqnarray}
  \hat{\bm{P}} &=& \frac{1}{C} \sum_{c = 1}^C \bm{P}_c,\\
  \hat{\bm{P}}' &=& \frac{\hat{\bm{P}} - \min(\hat{\bm{P}})}{\max(\hat{\bm{P}}) - \min(\hat{\bm{P}})},
\end{eqnarray}
where $\bm{P}_c \in \mathbb{R}^{H \times W}$ is the $c$-th channel of $\bm{F}$, $\min(\cdot)$ and $\max(\cdot)$ represent the calculation of the minimum value and maximum value of the input feature maps.

Through visualizations of the generated feature maps $\hat{\bm{P}}'$, we find some patterns on the activation regions of TF-HEAD, RetinaNet, FCOS, and Faster R-CNN. RetinaNet responds to regions where the semantic information is rich and beneficial to object classification, \eg side of the train and the zebra streaks. FCOS concentrates on the object boundaries like the last coach of the train and the horse legs. Faster R-CNN mainly responds to the center of the objects, with the rest parts of the object inactivated. Our HEAD framework achieves the most informative activation by aggregating feature extraction abilities from assistant detectors.
