# Supplementary material for: HEAD: HEtero-Assists Distillation for Heterogeneous Object Detectors
Source: arXiv:2207.05345 source file (2022-07-12)
Supplement: Supplementary file 4 [file code.tex]

We implement our method on mmdetection~\cite{mmdetection}. To replicate our work, first install mmdetection according to their official guide. Once mmdetection is successfully installed, use the files under the \verb|code| folder in the supplementary material to update the corresponding files under the mmdetection base directory. Note that some files, e.g. the todd directory, may not exist in the mmdetection base directory. Simply copy these files to the corresponding location in the mmdetection base directory. Finally, install the dependencies listed in \verb|requirements.txt|. To avoid version conflicts, we recommend to use mmdetection with git version \verb|ff9bc399| and manually build mmcv-full from git version \verb|366c628a|.

We provide two configs for replication: \verb|configs/kd/head_faster_r18.py| and \verb|configs/kd/head_faster_r18_dag.py|. Both configs use R18 RetinaNet as the student and R50 Faster R-CNN as the teacher. 

\verb|configs/kd/head_faster_r18.py| performs HEAD and is expected to reach $36.2$ mAP. 
\verb|configs/kd/head_faster_r18_dag.py| performs AKD only and is expected to reach $35.5$ mAP.
