# Supplementary material for: HEAD: HEtero-Assists Distillation for Heterogeneous Object Detectors
Source: arXiv:2207.05345 source file (2022-07-12)
Supplement: Supplementary file 5 [file overview.tex]

In the following sections, we provide additional information on our proposed HEAD and TF-HEAD frameworks. \Cref{sec:supp-takd} discusses the similarities and differences between our method and other knowledge distillation (KD) approaches with assistants. \Cref{sec:supp-proposals} details the procedure of generating proposals with one-stage students. \Cref{sec:supp-vis} demonstrates the characteristics of heterogeneous detectors through visualization. Finally, \cref{sec:supp-code} introduces the process of reproducing our work in detail.
